# Supplementary material for: Flying with Photons: Rendering Novel Views of Propagating Light
Source: arXiv:2404.06493 source file (2024-08-22)
Supplement: Supplementary file 1 [file supplement.pdf]

——— Supplementary Material ———
# Flying with Photons: Rendering Novel Views of Propagating Light

Anagh Malik[1,2⋆] Noah Juravsky[1] Ryan Po[3]
Gordon Wetzstein[3] Kiriakos N. Kutulakos[1,2] David B. Lindell[1,2]

[1]University of Toronto [2]Vector Institute [3]Stanford University
anaghmalik.com/FlyingWithPhotons

## S1 Implementation details

### S1.1 Proposed Method

The proposed method builds on NerfAcc's [4] Instant-NGP implementation using an occupancy grid. We use a batch size of $2^{17}$ samples for the simulated dataset and $2^{16}$ samples for the captured dataset, where each batch aggregates samples along all rendered rays. For the occupancy grid we use a threshold of $10^{-2}$ for binarization. We preprocess the data by dividing by the factor given in Table S1 and Table S2, where these parameters are roughly the 90th percentile value of the transient video rendered or captured for a centered view of the scene. We then tonemap the data by clipping the transient video between the values of 0 and 1 and applying a gamma correction with $\gamma = 5$ for simulated data and $\gamma = 2$ for captured data. Overall, these parameters are selected to balance contrast and detail in the rendered transient videos.

### S1.2 Transient NeRF

We implement Transient NeRF using the NerfAcc framework based on the description provided by the Malik et al. [5], and the training procedure follows that of the proposed method, including using 500k iterations for optimization on simulated data and 1M iterations for optimization on captured data. Following the authors' description of the method, no proprocessing (i.e., gamma correction) of the data is applied. Following Malik et al. [5] we use the Mitsuba-based temporal filter for the simulated dataset.

We also modify the rendering procedure to account for the non-coaxial illumination and imaging setup used in our simulations. Specifically, during the ray marching procedure we (1) calculate the path length to each sample along the camera ray, (2) calculate the distance from that point to the point light source (ignoring occlusions), and (3) assign the corresponding time-resolved radiance to a transient bin that accounts for the round trip distance from the light source to the sample and to the camera.

⋆ anagh@cs.toronto.edu

### S1.3 K-Planes

We follow the original K-Planes [2] implementation, training each scene with a ray batch size of 4096. Each scene is trained for a total of 300,000 iterations; this number is obtained by scaling the training hyper-parameters from the original K-Planes implementation based on number of views and sequence length of our data. Due to the limited expressivity of the K-Planes architecture, we crop simulated and captured datasets in the time dimension. This prevents the architecture from allocating capacity to fit parts of the transient where nearly no photons are detected. For the simulated results, we crop the transients by identifying, across all viewpoints, the shortest contiguous time sequence in which a photon is detected in every transient video frame. We follow the original K-Planes implementation and set the spatial resolution of the feature grid to 64 and the temporal resolution to 25. For captured results, we train on the first 3000 time bins of each transient video. Since captured scenes are typically longer in time than simulated scenes, we increase the temporal resolution of the feature grid to 100.

### S1.4 Direct–Global Separation

Our method can be used for 3D visualization of direct and global components of light transport. To separate light into direct and global components, we use the following procedure. First, we pre-process the captured transient data to separate direct and global components by fitting a Gaussian mixture model (with 5 components) to the 1D temporal waveform of each transient video pixel for all viewpoints. We use the implementation of `scikit-learn` [7] to fit the mixture. To identify the direct component, we perform a normalized cross-correlation between the fitted Gaussian mixture and the calibrated response of picosecond laser and SPAD to a direct reflection from a diffuse target. We identify if the maximum value of the normalized cross-correlation exceeds a threshold and, if so, the direct component is taken to be all Gaussians whose mean is less than the argmax of the normalized cross-correlation. Then, we set the indirect component to the remaining Gaussians. Alternatively, if no direct component is detected (i.e., the normalized cross-correlation does not exceed the threshold), the indirect component is taken to be the entire mixture of Gaussians. We set the threshold to 0.5 and find that this provides adequate selectivity for the direct component. Finally, we train separate instances of our model on the direct and global components, enabling synthesis of direct and global transient videos from novel viewpoints (see supplemental video).

## S2 Evaluation metrics

### S2.1 Transient IoU

We introduce the transient intersection-over-union (IoU) metric. This metric calculates the overlap between two time-resolved waveforms (i.e., transients) and

hence provides a measure of their similarity. Here, the intersection corresponds to the overlapping area of the two transients, and the union is the area when the greater of the transients at each time bin is considered. We assume that both transients are non-negative. The IoU is then calculated as the ratio of the intersection to the union of the histograms. Mathematically, it can be expressed as:

$$\mathrm{IoU}(\boldsymbol{\tau}_1, \boldsymbol{\tau}_2) = \frac{\sum_n \min\left(\boldsymbol{\tau}_1[n], \boldsymbol{\tau}_2[n]\right)}{\sum_n \max\left(\boldsymbol{\tau}_1[n], \boldsymbol{\tau}_2[n]\right)}, \tag{S1}$$

where $\tau_1, \tau_2$ are the transients being compared. The IoU metric ranges from 0 to 1, with a value of 1 indicating perfect overlap and complete similarity between the two histograms, while a value of 0 indicates no overlap and complete dissimilarity.

### S2.2 PSNR, LPIPS and SSIM

To calculate the image metrics, we need a 2D representation of our transient. To arrive at this representation, we take the integrated transient output for each method (over the time dimension), this gives a raw image, which is then scaled and clipped between 0 and 1. After that the images are gamma corrected with $\gamma = 2.2$. These images are then compared for PSNR, LPIPS and SSIM. The scales are shared between all methods and are fixed per dataset.

## S3 Dataset

The exact details of all the simulated and captured datasets can be found in Table S1 and Table S2 respectively.

*Illumination and detector configuration.* While both datasets use a static illumination source, future work could investigate scanning both the illumination source and the detector. However, capturing this type of data would require a more sophisticated gantry and longer acquisition times. Alternatively, our capture system supports using a static camera and scanned light source, which could enable applications in transient relighting.

**Table S1:** Descriptions of simulated scenes. All scenes have a test set of 60 test images.

| | scene description | training views | azimuth span | elevation span | bin width | normalization scale |
|---|---|---|---|---|---|---|
| Cornell box | A light source from the top illuminates two boxes, highlighting interreflections. | 93 | 180° | 45° | 0.1 | 43 |
| Peppers | A point light source from the top illuminates a glass ball and two peppers, red and green. The scene highlights refractions. | 93 | 45° | 30° | 0.02 | 5 |
| Pots | A point light source from the top illuminates a ficus and stacked pots, which are in front of a glass pillar. This scene highlights interreflections, refractions and shows more complicated geometry. | 93 | 90° | 30° | 0.02 | 500 |
| Caustics | A volume filled with smoke contains a point light source and a glass ball. The glass ball focuses the light which leaves the point source. | 45 | 45° | 15° | 0.05 | 20 |

**Table S2:** Descriptions of the captured scenes. All scenes have a calibrated bin width of 0.0105 m and span 15 degrees in elevation angle.

| | scene description | training views | test views | azimuth span | normalization scale | exposure time (s) |
|---|---|---|---|---|---|---|
| Coke bottle | A collimated beam enters a coke bottle, it gets focused at the cap. | 36 | 9 | 360° | 1000 | 2000 |
| Kennedy | A points source illuminates a brass Kennedy statue, we also witness interreflections in a mirror in the scene. | 60 | 15 | 150° | 400 | 1000 |
| David | A point source illuminates a statue of David and two candles from the side. | 60 | 15 | 150° | 6000 | 1000 |
| Mirror | A fish tank filled with water and a bit of milk. A collimated beam enters the tank and gets reflected on to a diffuser by a mirror. | 36 | 9 | 90° | 1500 | 2000 |
| Diffraction | A fish tank filled with water and milk. A collimated beam enters the tank and gets diffracted by a grating. | 39 | 9 | 90° | 500 | 2000 |

# S4 Additional Results

## S4.1 Simulated Results

We provide additional results on the simulated dataset (see Fig. S1) and report metrics for each scene (Tables S3, S4, S5, S6). We observe similar trends as in the main text; the proposed method without propagation delay modeling and K-Planes [2] fail to reconstruct transients with correct timing. In scenes with more inter-reflections, these methods fail entirely. T-NeRF [5] fails to reconstruct global illumination components. While the proposed method without propagation delay yields strong results across the image quality metrics, we note that it is only the *integrated images* that appear correct; the transient has incorrect time shifts, which results in a lower transient IoU score for that method.

**Table S3:** PSNR (dB) results on the simulated scenes.

| | *Cornell box* | *peppers* | *pots* | *smoke* | mean ↑ |
|---|---|---|---|---|---|
| T-NeRF | 21.471 | 27.119 | 28.916 | 27.892 | 26.349 |
| K-Planes | 13.768 | 18.391 | 18.728 | 31.317 | 20.551 |
| w/o prop. delay | 13.271 | 28.080 | 29.448 | 40.367 | 27.791 |
| proposed | 33.746 | 28.634 | 32.695 | 36.783 | 32.965 |

**Table S4:** LPIPS results on the simulated scenes.

| | *Cornell box* | *peppers* | *pots* | *smoke* | mean ↓ |
|---|---|---|---|---|---|
| T-NeRF | 0.361 | 0.334 | 0.320 | 0.337 | 0.338 |
| K-Planes | 0.525 | 0.298 | 0.707 | 0.192 | 0.431 |
| w/o prop. delay | 0.495 | 0.321 | 0.345 | 0.175 | 0.334 |
| proposed | 0.211 | 0.247 | 0.292 | 0.239 | 0.247 |

**Table S5:** SSIM results on the simulated scenes.

| | *Cornell box* | *peppers* | *pots* | *smoke* | mean ↑ |
|---|---|---|---|---|---|
| T-NeRF | 0.871 | 0.890 | 0.926 | 0.861 | 0.887 |
| K-Planes | 0.629 | 0.738 | 0.341 | 0.954 | 0.666 |
| w/o prop. delay | 0.703 | 0.933 | 0.947 | 0.994 | 0.894 |
| proposed | 0.974 | 0.946 | 0.959 | 0.982 | 0.965 |

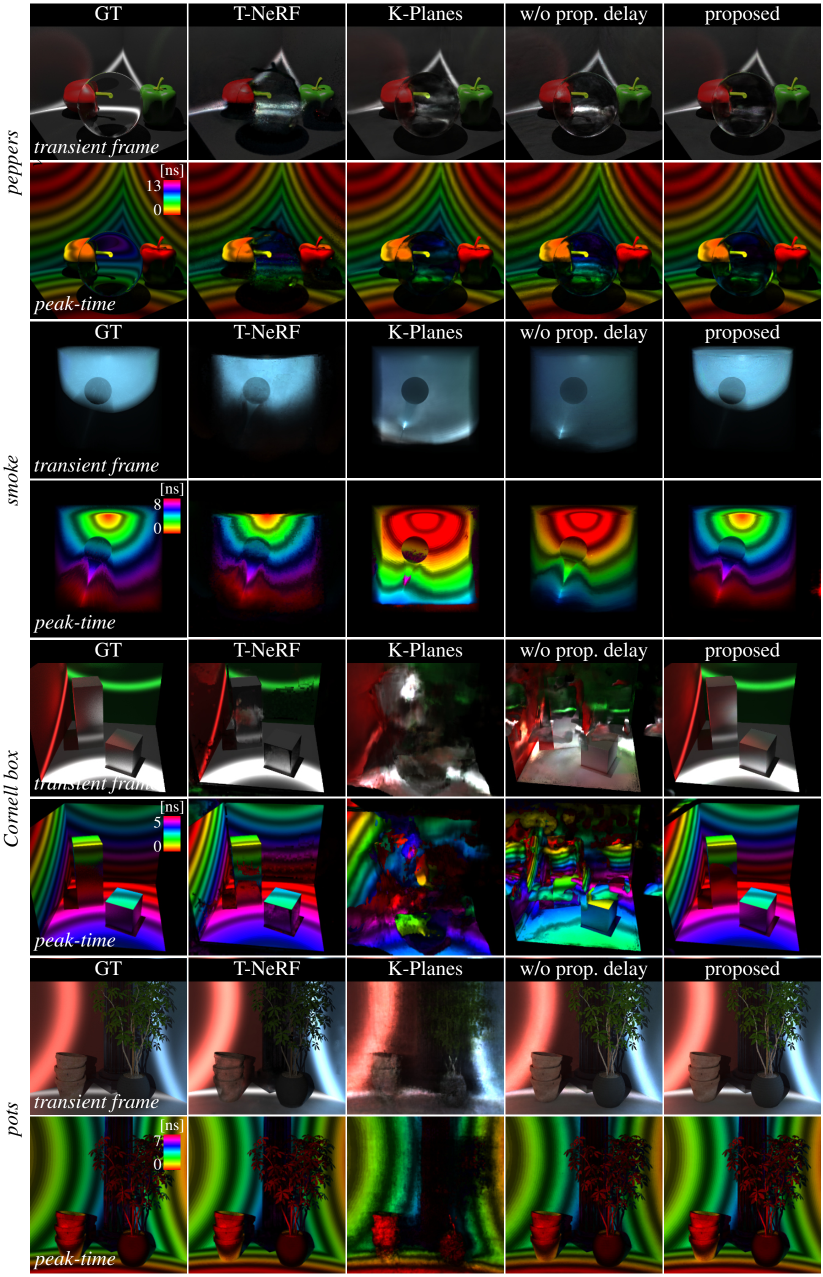


**Fig. S1:** Additional simulated results, transient frames and peak-time visualizations.

**Table S6:** Transient IoU results on the simulated scenes.

| | *Cornell box* | *peppers* | *pots* | *smoke* | mean ↑ |
|---|---|---|---|---|---|
| T-NeRF | 0.781 | 0.712 | 0.798 | 0.626 | 0.729 |
| K-Planes | 0.335 | 0.346 | 0.295 | 0.455 | 0.358 |
| w/o prop. delay | 0.185 | 0.360 | 0.456 | 0.472 | 0.368 |
| proposed | 0.915 | 0.722 | 0.858 | 0.824 | 0.830 |

## S4.2 Captured Results

We provide additional results on the captured dataset (see Figs. S2 and S3) and report metrics for each scene (Tables S7, S9, S8, S10). Again, we observe similar trends to the main text.

**Table S7:** PSNR (dB) results on the captured scenes.

| | *Coke bottle* | *Kennedy* | *David* | *mirror* | *diffraction* | mean ↑ |
|---|---|---|---|---|---|---|
| K-Planes | 20.979 | 20.690 | 29.810 | 27.060 | 22.035 | 24.635 |
| w/o prop. delay | 17.050 | 14.002 | 18.882 | 19.614 | 16.043 | 17.118 |
| proposed | 22.429 | 21.607 | 30.388 | 27.598 | 22.722 | 24.949 |

**Table S8:** SSIM results on the captured scenes.

| | *Coke bottle* | *Kennedy* | *David* | *mirror* | *diffraction* | mean ↓ |
|---|---|---|---|---|---|---|
| K-Planes | 0.519 | 0.561 | 0.433 | 0.511 | 0.559 | 0.506 |
| w/o prop. delay | 0.504 | 0.526 | 0.506 | 0.531 | 0.580 | 0.529 |
| proposed | 0.414 | 0.410 | 0.364 | 0.461 | 0.506 | 0.431 |

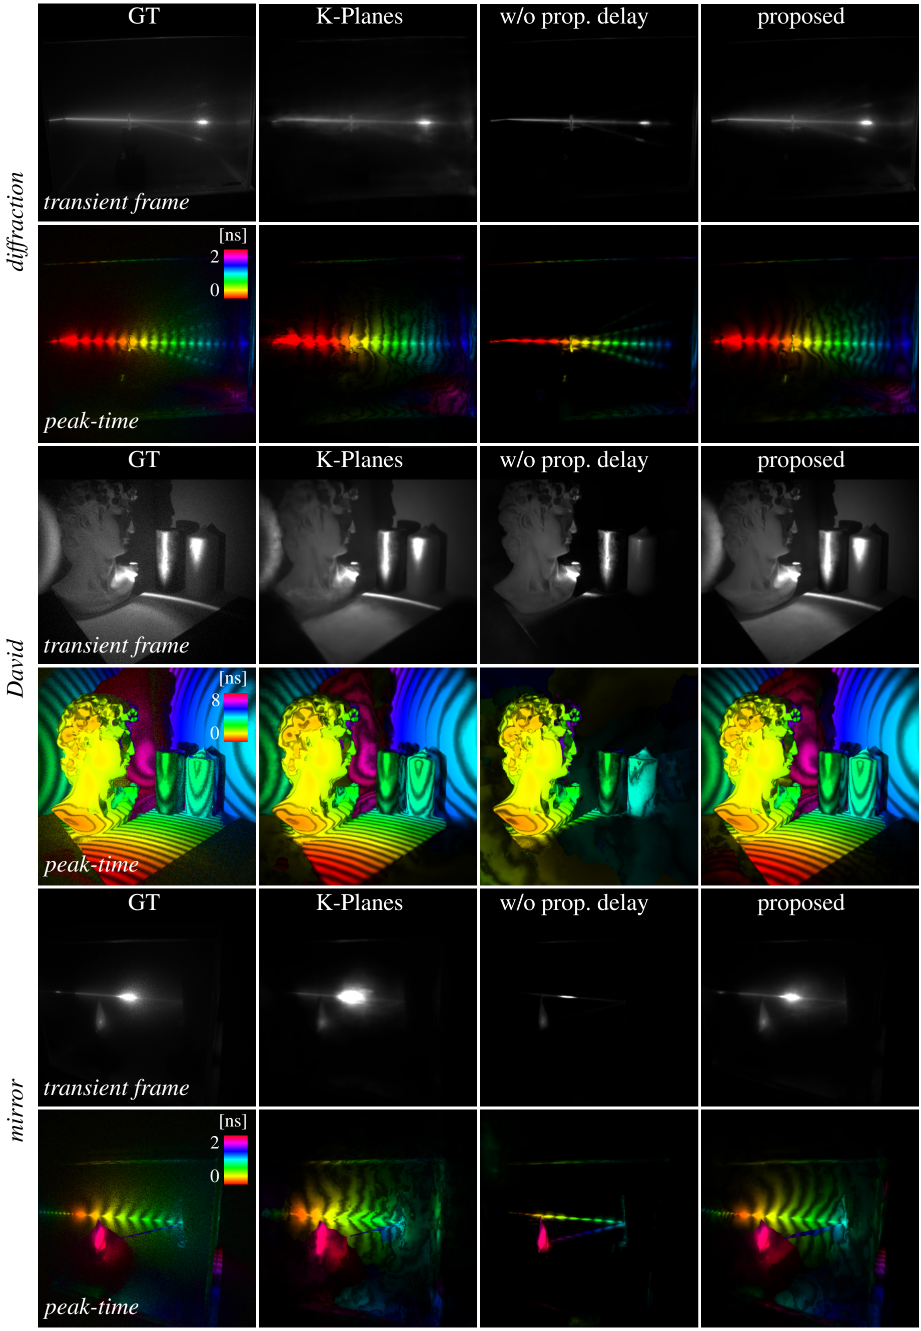


**Fig. S2:** Additional captured results, transient frames, and peak-time visualizations.

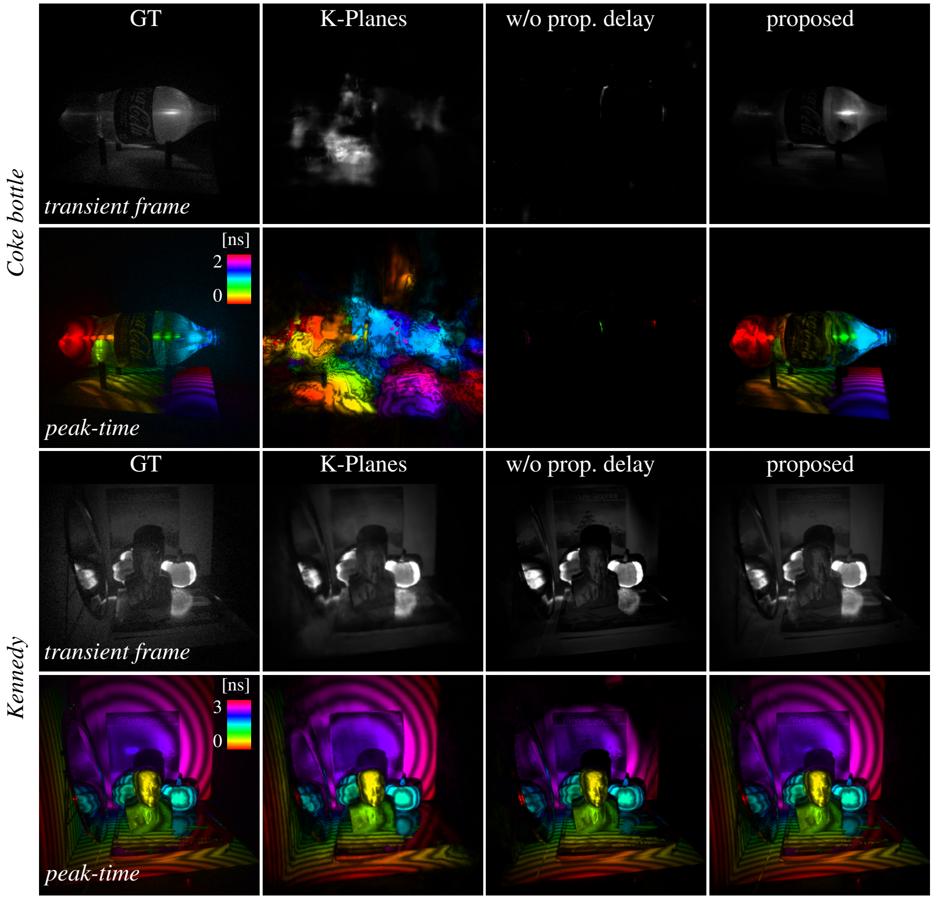


**Fig. S3:** Additional captured results, transient frames, and peak-time visualizations.

**Table S9:** LPIPS results on the captured scenes.

| | *Coke bottle* | *Kennedy* | *David* | *mirror* | *diffraction* | mean ↑ |
|---|---|---|---|---|---|---|
| K-Planes | 0.430 | 0.654 | 0.764 | 0.598 | 0.525 | 0.612 |
| w/o prop. delay | 0.200 | 0.438 | 0.438 | 0.403 | 0.251 | 0.346 |
| proposed | 0.351 | 0.774 | 0.876 | 0.717 | 0.611 | 0.666 |

**Table S10:** Transient IoU results on the captured scenes.

| | *Coke bottle* | *Kennedy* | *David* | *mirror* | *diffraction* | mean ↑ |
|---|---|---|---|---|---|---|
| K-Planes | 0.118 | 0.492 | 0.580 | 0.435 | 0.351 | 0.406 |
| w/o prop. delay | 0.002 | 0.359 | 0.336 | 0.052 | 0.119 | 0.174 |
| proposed | 0.298 | 0.574 | 0.607 | 0.460 | 0.399 | 0.468 |

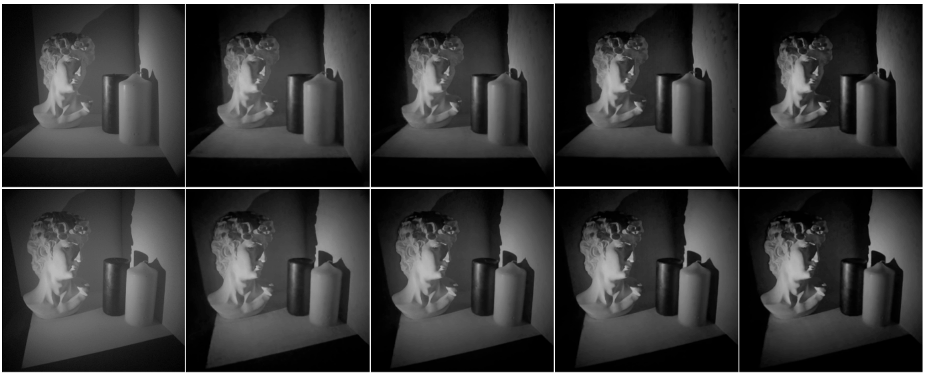


**Fig. S4:** Integrated transient videos rendered from novel views trained using transients with different light levels on the *David* scene. The method is trained on different subsets of the photon counts collected within the indicated exposure times per each view; at low photon count settings, the method struggles to reconstruct darker regions due to the low signal-to-noise ratio.

**Table S11:** Reconstruction quality vs. exposure time for the *David* scene. We report image quality metrics and Transient IoU for the proposed method trained on transient videos captured with varying exposure times.

| | PSNR ↑ | LPIPS ↓ | SSIM ↑ | Transient IoU ↑ |
|---|---|---|---|---|
| 100s | 24.030 | 0.391 | 0.683 | 0.512 |
| 250s | 26.173 | 0.372 | 0.779 | 0.564 |
| 500s | 27.971 | 0.355 | 0.848 | 0.578 |
| 1000s | 30.388 | 0.364 | 0.876 | 0.607 |

## S4.3 Noise Analysis

We conduct an experiment involving variations in the exposure time, specifically, we train the proposed method using the photons captured within one-half, one-tenth, and one-quarter of the original exposure time. This translates to an exposure time of $500s, 250s, 100s$ respectively, per each transient video. As expected, the reconstruction quality degrades somewhat with decreasing photon counts for all metrics (see Tab. S11). While the method performs worse in darker regions (which have lower signal-to-noise ratio) as the exposure time decreases, the main scene details are still accurately reconstructed even at the lowest exposure setting.

## S4.4 Ablation Studies

*Effect of tonemapping.* In Table S12, we compare tonemapping the ground truth using a gamma function vs. tonemapping the ground truth and the rendered data

**Table S12:** Evaluation of transient rendering from novel views.

| | method | param. | PSNR (dB) ↑ | LPIPS ↓ | T-IOU ↑ |
|---|---|---|---|---|---|
| *sim* | K-Planes $\gamma = 1$ | 37M | 17.519 | 0.564 | 0.245 |
| | K-Planes $\gamma = 5$ | 57M | 20.038 | 0.433 | 0.352 |
| | K-Planes $\gamma = 5$ | 37M | 20.551 | 0.431 | 0.358 |
| *sim* | Ours, $\gamma = 1$ | 15M | 28.224 | 0.414 | 0.695 |
| | Ours, $\gamma = 5$ | 15M | 32.965 | 0.247 | 0.830 |
| | Ours, RAWNeRF ($\gamma = 5$) | 15M | 34.692 | 0.212 | 0.861 |
| *cap* | Ours, $\gamma = 2$ | 15M | 24.949 | 0.431 | 0.468 |
| | Ours, RAWNeRF ($\gamma = 2$) | 15M | 24.835 | 0.534 | 0.302 |

in the loss function (as in RAWNeRF [6]) vs. using a linear mapping ($\gamma = 1$), and we report average performance for the simulated ("sim") and captured scenes ("cap"). We observe that (1) tonemapping improves performance over a linear mapping for both our method and K-Planes (all rows); (2) tonemapping both the renders and the measurements improves performance in simulation but not for captured data, where the model seems more sensitive to fitting noise (rows 5–6, 7–8).

*K-Planes parameters.* We attribute the lower performance of K-Planes relative to our approach to its lack of propagation delay modeling. The results are relatively insensitive to the parameter count—see Table S12, rows 2–3. Specifically, we re-ran K-Planes on the simulated dataset after increasing the parameter count from 37M to 57M (more than the K-Planes models that we used for captured data, whose transients have more time bins). We observe a small change in performance; the slight ($\approx$ 0.5 dB) drop in the PSNR of novel views could be due to a tendency for increased overfitting to training viewpoints with more parameters.

### S4.5 Time Warping

Our approach can be used to visualize light transport in different ways through time warping, which involves adding or removing time delays to the rendered transients. Following Velten et. al [8] we perform depth-based time warping, which removes the propagation delay from the scene point to the camera. In the visualization with depth-based warping, points along each camera ray "light up" as soon as they intersect a wavefront of light; in other words, each camera ray is rendered in a different spacetime coordinate frame. To create this visualization, we calculate the propagation delay to each scene point using the expected ray termination distance [1], and we shift the rendered transient by the corresponding speed-of-light time delay. We compare transients rendered with and without depth-based warping in Fig. S5.

Our representation enables more general time warping techniques, wherein we shift the transients based on the distance to arbitrary reference surfaces

(e.g., defined by a sphere, cube, etc.). We explore extensions to time warping and associated novel visualization techniques in Figure. S5, specifically, we show sphere, cube, back-sphere and back-cube warpings for the *Cornell box* scene.

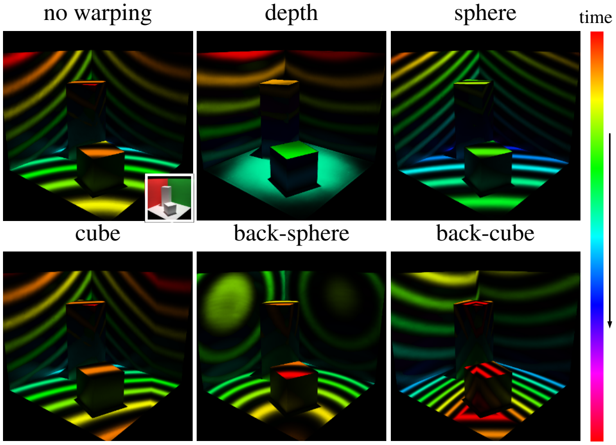


**Fig. S5:** Visualization of different methods for time warping.

To perform the sphere warping each transient is shifted by the distance between the camera origin and a sphere that encapsulates the scene. Using the sphere surface as the spacetime reference frame reduces view-dependent changes in the appearance of the scene, especially as the scene–camera distance increases. Rather than shifting the transient by the distance between the camera origin and the sphere, we can instead shift by the distance between the camera origin and the second intersection with the sphere; we call this the back-sphere warping. This method for warping accentuates the curvature of propagating wavefronts. We can similarly visualize wavefronts using a spacetime reference frame corresponding to the surface of a cube that encapsulates the scene. Then, we can shift the transients by the distance from the camera center of projection to the near surface of the cube (cube warping) or the far surface of the cube (back-cube warping).

## S4.6 Relativistic Rendering

To create the relativistic visualizations we reimplement the relativistic rendering procedures of Jarabo et al. [3]. We now explain how we implement the relativistic effects, shown in the main paper figures. Let the observer speed be given as $v = \beta c$, where $c$ is the speed of light and $\beta$ is a factor. Then we denote $\gamma = \frac{1}{(1-\beta^2)^{1/2}}$.

*Camera deformation.* This effect is caused by the Lorentz contraction; here the camera field of view changes based on the camera velocity. To implement the camera deformation we augment the camera's field of view. Specifically let $f_x, f_y$ be the focal lengths in the horizontal and vertical directions, then the new camera focal lengths are given as $f_x^{'} = \frac{f_x}{\gamma}$ and $f_y^{'} = \frac{f_y}{\gamma}$.

*Relativistic aberration.* This operation warps the camera rays based on the camera velocity. Specifically, let also $v$ be the camera ray vector and $M$ the velocity vector of the observer. Then $\theta$ is the angle between them, due to relativity this angle gets changed. In particular, the new angle is given through its cosine:

$$\cos(\theta^{'}) = \frac{\cos(\theta) - \beta}{1 - \beta cos(\theta)}. \tag{S2}$$

*Time dilation.* This operation shifts and stretches the transients in time. The exact equations for these warpings are provided by Jarabo et al. [3] (see their Eq. 3, and Eq. 11).

*Searchlight effect.* This operation applies a spatial modulation to the intensity of light based on the camera velocity. Let $D = \gamma(1 + \beta\cos(\theta^{'}))$, where $\theta^{'}$ gives the warped rays' angles for the image as described in the *Relativistic aberration* section. Then the radiance of the ray is scaled by the factor $D^{-5}$ [3]. This results in increased brightness in the center of the image or the edges, depending on the direction of motion.

We do not implement Doppler shift [9] because the transient videos are captured using a narrowband pulsed laser (so no relative shift between wavelengths would be observed).

## References


1. Deng, K., Liu, A., Zhu, J.Y., Ramanan, D.: Depth-supervised NeRF: Fewer views and faster training for free. In: Proc. CVPR (2022)
2. Fridovich-Keil, S., Meanti, G., Warburg, F.R., Recht, B., Kanazawa, A.: K-Planes: Explicit radiance fields in space, time, and appearance. In: Proc. CVPR (2023)
3. Jarabo, A., Masia, B., Velten, A., Barsi, C., Raskar, R., Gutierrez, D.: Relativistic effects for time-resolved light transport. Computer Graphics Forum **34**, 1–12 (2015)
4. Li, R., Gao, H., Tancik, M., Kanazawa, A.: NerfAcc: Efficient sampling accelerates nerfs. arXiv preprint arXiv:2305.04966 (2023)
5. Malik, A., Mirdehghan, P., Nousias, S., Kutulakos, K.N., Lindell, D.B.: Transient neural radiance fields for lidar view synthesis and 3D reconstruction. In: Proc. NeurIPS (2023)
6. Mildenhall, B., Hedman, P., Martin-Brualla, R., Srinivasan, P.P., Barron, J.T.: NeRF in the dark: High dynamic range view synthesis from noisy raw images. In: Proc. CVPR (2022)
7. Pedregosa, F., Varoquaux, G., Gramfort, A., Michel, V., Thirion, B., Grisel, O., Blondel, M., Prettenhofer, P., Weiss, R., Dubourg, V., Vanderplas, J., Passos, A., Cournapeau, D., Brucher, M., Perrot, M., Duchesnay, E.: Scikit-learn: Machine learning in Python. J. Mach. Learn. Res. **12**, 2825–2830 (2011)
8. Velten, A., Wu, D., Jarabo, A., Masia, B., Barsi, C., Joshi, C., Lawson, E., Bawendi, M., Gutierrez, D., Raskar, R.: Femto-photography: Capturing and visualizing the propagation of light. ACM Trans. Graph. **32**(4), 1–8 (2013)
9. Weiskopf, D., Kraus, U., Ruder, H.: Searchlight and Doppler effects in the visualization of special relativity: A corrected derivation of the transformation of radiance. ACM Trans. Graph. **18**(3), 278–292 (1999)
